# Supplementary material for: Robust Surgical Phase Recognition From Annotation Efficient Supervision
Source: arXiv:2406.18481 source file (2024-06-26)
Supplement: Supplementary file 1 [file 7_supp.tex]

% \subsection{Explanation about CTC and STC}
% \label{subsec:ctc}
% Connectionist Temporal Classification (CTC) loss aims to tackle misalignment between input and output sequences of varying lengths, and is widely used for automatic speech recognition \cite{li2022recent} and handwritten text
% recognition.
% \cite{alkendi2024advancements}.
% Assuming we are given a video X containing T frames and a full labeling y$y\in \mathcal{P}^N$, where N is the labeling length.
% The CTC adds an additional $blank$ token
% and a function $B(\cdot)$ that maps frame-wise predictions to dense predictions by removing $blank$ tokens and repeating predictions.

% The CTC loss can be expressed as follows:
% \begin{align}
%     \mathcal{L_{CTC}} 
%         &= - ln \, P(y|X) \\
%         &= - ln \, \sum\limits_{\{\pi | B(\pi) = y\}} P(\pi| X)
% \end{align}
% where $\pi$ represents a sparse prediction that would have collapsed to the correct labeling.
% Using the CTC's assumption of 
% conditional independence
% \begin{equation}
%     P(\pi| X) = \prod\limits_{t=1}^{T} P(\pi_t|t, X) 
% \end{equation}
% $P(\pi_t|t, X)$ are given by the model. 
% This loss can be efficiently calculated using dynamic programming.
% CTC can also be calculated using weighted finite-state transducers \cite{hannun2020differentiable}.
% STC \cite{pratap2022star} is a variation of the CTC loss aiming to allow learning from weakly supervised labels. The STC is based on adding an additional $star$ token that can represent a missing label. This idea allows handling of a flexible number of missing tokens.  

% \subsection{Temporal metrics}
% Edit score was introduced by Lea \etal \cite {lea2016learning} and is based on the Levenshtein distance (also edit known as  distance) which is equal to the number of insertions, replacements, and deletions of letters needed to convert one string to another.
% Given a segmental labeling P and ground truth GT,
% the edit score is calculated as
% \begin{equation}
%     Edit \; score = 1 - \frac{L(P, GT)}{max(|P|, |GT|)}
% \end{equation}
% where $L(\cdot, \cdot)$ denotes the Levenshtein distance.

% F1@k metrics was proposed by Lea \etal \cite{lea2017temporal}. They are based on intersection over union (IoU) measures between the prediction segments, the ground truth segments, and a corresponding threshold for each metric.  
